# Supplementary material for: Dynamic Memory based Attention Network for Sequential Recommendation
Source: arXiv:2102.09269 source file (2021-02-18)
Supplement: Supplementary file 1 [file 6.appendix.tex]

% \appendix
\begin{table*}[htpb]
\centering
\small
  \caption{Efficiency analysis for all models (in seconds per 1024 users). }
  \begin{tabular}{c|ccccccc}
    \hline
     &\textbf{GRU4Rec} &\textbf{Caser} &\textbf{SASRec} &\textbf{SHAN} &\textbf{SDM} &\textbf{HPMN} &\textbf{DMAN}\\
    \hline
    \textbf{Taobao} &0.811 &0.772 &0.613 &0.716 &0.733 &0.358 (1st) &0.439 (2nd)\\
    \hline
    \textbf{XLong} &2.447 &2.283 &1.783 &1.523 &1.866 &0.362 (1st) &0.442 (2nd)\\
  \hline
\end{tabular}
\label{table1}
\end{table*}
\section{Appendix for Experiment Setup}
In this section, we give more descriptions of the datasets used in the paper. Besides, we also introduce the hyper-parameter configurations of baseline methods.

\subsection{Dataset Details}
We conduct experiments on four publicly accessible benchmark datasets to evaluate the effectiveness of the proposed model. 

\textbf{MovieLens}~\footnote{https://grouplens.org/datasets/movielens/1m/} is a popular movie rating dataset. Similar to~\cite{he2016fast}, we transform the rating scores into binary values; each entry is either 1 or 0, indicating whether the user rated the movie. The 1M version is used in our experiments.

\textbf{Taobao}~\footnote{https://tianchi.aliyun.com/dataset/dataDetail?dataId=649} is a dataset of user behaviors from the commercial platform of Taobao~\cite{zhu2018learning}. It consists of one million users' user behavior activities from November 25 to December 3, 2017, where each log records the user ID, item ID, category ID, behavior type, and action timestamp. There are four types of behaviors, including purchase, cart, item favoring, and click actions. 

\textbf{JD}~\footnote{http://www.jd.com} is a collection of user browsing logs over e-commerce products collected from the JD website. It contains several types of user behaviors from March 15 to April 15, 2018. Following the preprocessing of~\cite{lv2019sdm}, we treat different types of actions as click interaction and target to predict whether the user will click the item.

\textbf{XLong}~\footnote{https://tianchi.aliyun.com/dataset/dataDetail?dataId=22482} is a user behavior dataset sampled from the click logs of more than twenty thousand users on Alibaba e-commerce platform from April to September 2018~\cite{ren2019lifelong}. It is the longest public dataset that has more than one thousand historical interactions per user on average. Thus, it is more challenging to process than other datasets. 

For the four datasets above, we only keep users who have interacted with more than ten items.

\subsection{Implementation Configuration}
The codes of all baseline methods are released online. For a fair comparison, all methods are implemented in Tensorflow and optimized with Adam optimizer with a mini-batch size of 128. We tune the parameters of comparing methods according to values suggested in original papers and set the embedding size as 128 and the number of negative samples as 5 for all methods. For training, we run experiments on 5 parameter severs (PSs) and 6 GPU (Tesla P100-PCIE-16GB) workers. Specifically, experimental configurations for baselines are tuned as below. 
\begin{itemize}
\item \textbf{Traditional Sequential methods}: For Caser~\cite{tang2018personalized}, the number of the vertical and horizontal filters are searched from $\{1,2,4,8,16,32,64\}$ based on NeuRec Library~\footnote{https://github.com/wubinzzu/NeuRec}. For SASRec~\cite{kang2018self}, the number of self-attention blocks is searched from $\{1,2,3,4,5\}$. 

\item \textbf{Long sequential methods}: 
For {SDM}~\cite{lv2019sdm}, the number of self-attention heads are searched from $\{2,4,8,10,12,14,16\}$. For {SHAN}~\cite{ying2018sequential}, the item embedding regularization weight $\lambda_{uv}$ and attention network regularization $\lambda_a$ are searched from $\{0.0001, 0.001, 0.01 \}$ and $\{0, 1, 10, 50\}$, respectively.
For HPMN~\cite{ren2019lifelong}, the regularization weight $\lambda$ and $\mu$ are searched from $\{1\times 10^{-3}, 1\times 10^{-4}, 1\times 10^{-5}\}$; the number of layers and update periods are selected from $\{2,3,4,5,6,\}$ and $\{1,2,4,8,16,32\}$. 
\end{itemize}

For the proposed method, the number of memory slots $m$ and attention layers $L$ are searched from $\{2,4,6,8,10,20,30\}$ and $\{1,2,3,4,5\}$, respectively.

\subsection{Efficiency Evaluation}
We also compare the running time cost of all methods to verify the efficiency of the proposed method. Specifically, we record the GPU time of all models to generate embeddings for 1024 users in the forward pass. We conduct experiments based on a Linux system with 24 Intel(R) Xeon(R) CPU E5-2650 v4\@2.2GHz processors and 4 GeForce GTX-1080 Ti 12 GB GPU. Table~\ref{table1} reports the results on two representative datasets. Note that the results on MovieLens and JD.com datasets should be similar to that of Taobao dataset, since they have the same maximum user behavior sequence.   

From Table~\ref{table1}, we can observe that our model runs faster than all other baselines, excepting HPMN. Specifically, the difference gap between DMAN and other methods on XLong dataset is significantly larger than that on Taobao dataset. This result shows that our model is efficient to handle longer user behavior sequence. HPMN utilizes a memory network to cache both short-term and long-term interests for next-item prediction, so it runs faster than our model. In theory, three traditional sequential models (GRU4Rec, Caser, and SASRec) and two long sequential models (SHAN and SDM) require to process $N\times{T}$ behavior sequence for inference, while HPMN needs to process $m$ memory blocks only. For our model, it requires to process $m$ memory blocks plus $2T$ short-term behavior sequence in total for user profiling. Considering the substantial improvements of our model compared with HPMN in terms of accuracy, DMAN is more suitable for user modeling with long behavior sequence.
